# Supplementary material for: Symmetry dictated universal helicity redistribution of Dirac fermions in transport
Source: arXiv:2309.02474 source file (2023-09-30)
Supplement: Supplementary file 1 [file SM.pdf]

# Supplemental Material: Symmetry dictated universal helicity redistribution of Dirac fermions in transport

Jun-Yin Huang,[1] Rui-Hua Ni,[1] Hong-Ya Xu,[1,*] and Liang Huang[1,†]

[1]*Lanzhou Center for Theoretical Physics, Key Laboratory of Theoretical Physics of Gansu Province, and Key Laboratory for Quantum Theory and Applications of the Ministry of Education, Lanzhou University, Lanzhou, Gansu 730000, China*

**CONTENTS**

I. The transfer matrix method for solving the transport problem 2
A. Numerical procedure to solve the piecewise-constant potential model with $n$ regions 2
B. Numerical result vs analytical result for a linear electrostatic potential 5

II. Analytical solution of the model with 3 regions 6

III. The universal helicity redistribution rule in the electrostatic potential case 7
A. The rule dictated by one-parameter transformation group of Lorentz boost $\Lambda(w)$ 7
B. The rule in Klein tunneling regime dictated by complex Lorentz boost $\Lambda(\mathrm{i}\pi)\Lambda(w)$ 9

IV. The universal helicity redistribution rule in the mass potential case dictated by $\Gamma(\mu)$ 11

References 12

* Corresponding author: xuhongya@lzu.edu.cn
† Corresponding author: huangl@lzu.edu.cn

## I. THE TRANSFER MATRIX METHOD FOR SOLVING THE TRANSPORT PROBLEM

### A. Numerical procedure to solve the piecewise-constant potential model with $n$ regions

For one-dimensional piecewise-constant electrostatic potential of arbitrary shape along the $x$-axis, the potential can in general be written as

$$V = \begin{cases} V_1 = 0, & x < x_1 (\equiv 0) \text{ (region 1)}, \\ V_2, & x_1 \leq x < x_2 \text{ (region 2)}, \\ \cdots & \cdots \\ V_j, & x_{j-1} \leq x < x_j \text{ (region } j), \\ \cdots & \cdots \\ V_n, & x \geq x_{n-1} (\equiv L) \text{ (region } n). \end{cases} \tag{S1.1}$$

The mass potential case can be written similarly as specified by the mass potential $U_j$ in region $j$. For an incident wave with energy $E$ and incident angles $\theta_1$ and $\varphi_1$, the momentum is then $p_1 = |\mathbf{p}_1| = \sqrt{E^2 - m^2}$, and the $y$ and $z$ components are $(p_y, p_z) = p_1(\sin\theta_1 \sin\varphi_1, \cos\theta_1)$, which are conserved due to the translational symmetry of the system in $y$ and $z$ directions. In region $j$, one has $p_j = \sqrt{(E - V_j)^2 - m^2}$ for the electrostatic potential case and $p_j = \sqrt{E^2 - (m + U_j)^2}$ for the mass potential case. The transmitted wavefunctions are plane wave solutions that can be chosen as the common eigenstates of $\hat{H}$, $\hat{\mathbf{p}}$, and $\hat{h}$ [1]

$$\psi_j^{(h)} = \begin{pmatrix} \chi_j^{(h)} \\ hk_j \chi_j^{(h)} \end{pmatrix} e^{\mathrm{i}(\mathbf{p}_j \cdot \mathbf{x} - Et)}, \tag{S1.2}$$

where $k_j = p_j/(E - V_j + m)$ for electrostatic potential and $k_j = p_j/(E + m + U_j)$ for mass potential, $h = \pm 1$ is the eigenvalue of $\hat{h}$, $\mathbf{p}_j = (p_{j,x}, p_y, p_z) = p_j(\sin\theta_j \cos\varphi_j, \sin\theta_j \sin\varphi_j, \cos\theta_j)$, and

$$\chi_j^{(+)} = [\cos\frac{\theta_j}{2} e^{-\mathrm{i}\varphi_j/2}, \sin\frac{\theta_j}{2} e^{\mathrm{i}\varphi_j/2}]^T,$$
$$\chi_j^{(-)} = [-\sin\frac{\theta_j}{2} e^{-\mathrm{i}\varphi_j/2}, \cos\frac{\theta_j}{2} e^{\mathrm{i}\varphi_j/2}]^T.$$

The corresponding angle parameters $\theta_j$ and $\varphi_j$ in spherical coordinates are

$$\theta_j = \cos^{-1}(p_1 \cos\theta_1 / p_j),$$
$$\varphi_j = \cos^{-1}\left(\lambda_j \sqrt{p_j^2 - p_y^2 - p_z^2} \Big/ p_j \sin\theta_j\right),$$

where $\lambda_j = \mathrm{sgn}(E - V_j)$ is for positive or negative energy states, respectively.

Then the wavefunction in region $j$ can be expanded on these bases with the coefficients $t_j^{(h)}$ and $r_j^{(h)}$ corresponding to transmitted and reflected terms, and the superscript "$(\pm)$" represents matching to the positive or negative helicity eigenstates: $\psi_j = t_j^{(h)} \psi_j^{(h)} + r_j^{(h)} \overline{\psi}_j^{(h)}$, with $\overline{\psi}_j^{(h)}$ the reflected eigen planewaves (from $\psi_j^{(h)}$ by replacing $p_{j,x}$ to $-p_{j,x}$ and $\varphi_j$ to $\pi - \varphi_j$). Without loss of generality, we assume that the incident Dirac fermions are completely positively helicity-polarized plane waves, i.e., $t_1^{(+)} = 1$, $t_1^{(-)} = 0$. A series of equations can be obtained by the continuity conditions for wavefunctions at the boundary between adjacent regions:

$$I \begin{pmatrix} 1 \\ 0 \\ r_1^{(+)} \\ r_1^{(-)} \end{pmatrix} = M_2 \cdot D_2' \begin{pmatrix} t_2^{(+)} \\ t_2^{(-)} \\ r_2^{(+)} \\ r_2^{(-)} \end{pmatrix}, \tag{S1.3}$$

$$M_j \cdot D_j \begin{pmatrix} t_j^{(+)} \\ t_j^{(-)} \\ r_j^{(+)} \\ r_j^{(-)} \end{pmatrix} = M_{j+1} \cdot D'_{j+1} \begin{pmatrix} t_{j+1}^{(+)} \\ t_{j+1}^{(-)} \\ r_{j+1}^{(+)} \\ r_{j+1}^{(-)} \end{pmatrix}, \tag{S1.4}$$

$$M_{n-1} \cdot D_{n-1} \begin{pmatrix} t_{n-1}^{(+)} \\ t_{n-1}^{(-)} \\ r_{n-1}^{(+)} \\ r_{n-1}^{(-)} \end{pmatrix} = T \begin{pmatrix} t_n^{(+)} \\ t_n^{(-)} \end{pmatrix}, \tag{S1.5}$$

where $D_j = \mathrm{diag}(e^{\mathrm{i}x_j p_{j,x}}, e^{\mathrm{i}x_j p_{j,x}}, e^{-\mathrm{i}x_j p_{j,x}}, e^{-\mathrm{i}x_j p_{j,x}})$, $D'_{j+1} = \mathrm{diag}(e^{\mathrm{i}x_j p_{j+1,x}}, e^{\mathrm{i}x_j p_{j+1,x}}, e^{-\mathrm{i}x_j p_{j+1,x}}, e^{-\mathrm{i}x_j p_{j+1,x}})$, and

$$I = e^{-\mathrm{i}\varphi_1/2} \begin{pmatrix} \cos\frac{\theta_1}{2} & -\sin\frac{\theta_1}{2} & -\mathrm{i}\cos\frac{\theta_1}{2}e^{\mathrm{i}\varphi_1} & \mathrm{i}\sin\frac{\theta_1}{2}e^{\mathrm{i}\varphi_1} \\ \sin\frac{\theta_1}{2}e^{\mathrm{i}\varphi_1} & \cos\frac{\theta_1}{2}e^{\mathrm{i}\varphi_1} & \mathrm{i}\sin\frac{\theta_1}{2} & \mathrm{i}\cos\frac{\theta_1}{2} \\ k_1\cos\frac{\theta_1}{2} & k_1\sin\frac{\theta_1}{2} & -\mathrm{i}k_1\cos\frac{\theta_1}{2}e^{\mathrm{i}\varphi_1} & -\mathrm{i}k_1\sin\frac{\theta_1}{2}e^{\mathrm{i}\varphi_1} \\ k_1\sin\frac{\theta_1}{2}e^{\mathrm{i}\varphi_1} & -k_1\cos\frac{\theta_1}{2}e^{\mathrm{i}\varphi_1} & \mathrm{i}k_1\sin\frac{\theta_1}{2} & -\mathrm{i}k_1\cos\frac{\theta_1}{2} \end{pmatrix}, \tag{S1.6}$$

$$M_j = e^{-\mathrm{i}\varphi_j/2} \begin{pmatrix} \cos\frac{\theta_j}{2} & -\sin\frac{\theta_j}{2} & -\mathrm{i}\cos\frac{\theta_j}{2}e^{\mathrm{i}\varphi_j} & \mathrm{i}\sin\frac{\theta_j}{2}e^{\mathrm{i}\varphi_j} \\ \sin\frac{\theta_j}{2}e^{\mathrm{i}\varphi_j} & \cos\frac{\theta_j}{2}e^{\mathrm{i}\varphi_j} & \mathrm{i}\sin\frac{\theta_j}{2} & \mathrm{i}\cos\frac{\theta_j}{2} \\ k_j\cos\frac{\theta_j}{2} & k_j\sin\frac{\theta_j}{2} & -\mathrm{i}k_j\cos\frac{\theta_j}{2}e^{\mathrm{i}\varphi_j} & -\mathrm{i}k_j\sin\frac{\theta_j}{2}e^{\mathrm{i}\varphi_j} \\ k_j\sin\frac{\theta_j}{2}e^{\mathrm{i}\varphi_j} & -k_j\cos\frac{\theta_j}{2}e^{\mathrm{i}\varphi_j} & \mathrm{i}k_j\sin\frac{\theta_j}{2} & -\mathrm{i}k_j\cos\frac{\theta_j}{2} \end{pmatrix}, \tag{S1.7}$$

$$T = e^{-\mathrm{i}\varphi_n/2} \begin{pmatrix} \cos\frac{\theta_n}{2} & -\sin\frac{\theta_n}{2} \\ \sin\frac{\theta_n}{2}e^{\mathrm{i}\varphi_n} & \cos\frac{\theta_n}{2}e^{\mathrm{i}\varphi_n} \\ k_n\cos\frac{\theta_n}{2} & k_n\sin\frac{\theta_n}{2} \\ k_n\sin\frac{\theta_n}{2}e^{\mathrm{i}\varphi_n} & -k_n\cos\frac{\theta_n}{2}e^{\mathrm{i}\varphi_n} \end{pmatrix} e^{\mathrm{i}x_{n-1}p_{n,x}}. \tag{S1.8}$$

The matrix $H_j$ is defined as

$$\begin{aligned} H_j &= M_j \cdot D'_j \cdot D_j^{-1} \cdot M_j^{-1} \\ &= \frac{1}{\cos\varphi_j} \begin{pmatrix} \cos(p_{j,x}d_j + \varphi_j) & g_j\cos\theta_j & 0 & g_j/k_j \\ -g_j\cos\theta_j & \cos(p_{j,x}d_j - \varphi_j) & g_j/k_j & 0 \\ 0 & g_jk_j & \cos(p_{j,x}d_j + \varphi_j) & g_j\cos\theta_j \\ g_jk_j & 0 & -g_j\cos\theta_j & \cos(p_{j,x}d_j - \varphi_j) \end{pmatrix}, \end{aligned} \tag{S1.9}$$

where $j = 2, 3, ..., n-2$, $d_j = x_j - x_{j-1}$ is the width of the $j$-th region, and $g_j = -\mathrm{i}\sin(p_{j,x}d_j)/\sin\theta_j$.

Thus Eqs. (S1.3)–(S1.5) can be simplified to

$$I \begin{pmatrix} 1 \\ 0 \\ r_1^{(+)} \\ r_1^{(-)} \end{pmatrix} = H_2 \cdot H_3 \cdots H_{n-1} \cdot T \begin{pmatrix} t_n^{(+)} \\ t_n^{(-)} \end{pmatrix} \tag{S1.10}$$

where the reflection and transmission coefficients can be figured out by numerically solving Eq. (S1.10). The overall transmission and reflection probabilities are then

$$\begin{aligned} T^{(h)} &= |t_n^{(h)}|^2 k_n \sin\theta_n \cos\varphi_n \big/ k_1 \sin\theta_1 \cos\varphi_1, \\ R^{(h)} &= |r_1^{(h)}|^2, \end{aligned} \tag{S1.11}$$

following $T^{(+)} + T^{(-)} + R^{(+)} + R^{(-)} = 1$ in terms of the probability current conservation.

For arbitrary given region $j$, the coefficients $t_j^{(h)}$ and $r_j^{(h)}$ can be calculated numerically too. Following the above procedures, we utilize the continuity conditions for the wavefunction at $x > x_j$, and then obtain the equation

$$\begin{pmatrix} t_j^{(+)} \\ t_j^{(-)} \\ r_j^{(+)} \\ r_j^{(-)} \end{pmatrix} = D_j^{-1} \cdot M_j^{-1} \cdot H_{j+1} \cdot H_{j+2} \cdots H_{n-1} \cdot T \begin{pmatrix} t_n^{(+)} \\ t_n^{(-)} \end{pmatrix}$$

with $t_n^{(h)}$ solved from Eq. (S1.10), and

$$M_j^{-1} = \frac{e^{\mathrm{i}\varphi_j/2}}{4\cos\varphi_j} \begin{pmatrix} e^{-\mathrm{i}\varphi_j}/\cos\frac{\theta_j}{2} & 1/\sin\frac{\theta_j}{2} & e^{-\mathrm{i}\varphi_j}/k_j\cos\frac{\theta_j}{2} & 1/k_j\sin\frac{\theta_j}{2} \\ -e^{-\mathrm{i}\varphi_j}/\sin\frac{\theta_j}{2} & 1/\cos\frac{\theta_j}{2} & e^{-\mathrm{i}\varphi_j}/k_j\sin\frac{\theta_j}{2} & -1/k_j\cos\frac{\theta_j}{2} \\ \mathrm{i}/\cos\frac{\theta_j}{2} & -\mathrm{i}e^{-\mathrm{i}\varphi_j}/\sin\frac{\theta_j}{2} & \mathrm{i}/k_j\cos\frac{\theta_j}{2} & -\mathrm{i}e^{-\mathrm{i}\varphi_j}/k_j\sin\frac{\theta_j}{2} \\ -\mathrm{i}/\sin\frac{\theta_j}{2} & -\mathrm{i}e^{-\mathrm{i}\varphi_j}/\cos\frac{\theta_j}{2} & \mathrm{i}/k_j\sin\frac{\theta_j}{2} & \mathrm{i}e^{-\mathrm{i}\varphi_j}/k_j\cos\frac{\theta_j}{2} \end{pmatrix}. \tag{S1.12}$$

Therefore, all the coefficients can be computed. Or similarly, we can utilize $r_1^{(h)}$ and the continuity conditions at $x \le x_j$.

For transmitted flow, the helicity polarization is defined as

$$P_j = (J_j^{(+)} - J_j^{(-)})/(J_j^{(+)} + J_j^{(-)}), \tag{S1.13}$$

where $J_j^{(h)} = |t_j^{(h)}|^2 |\psi_j^{(h)\dagger} \boldsymbol{\alpha} \psi_j^{(h)}|$ is the magnitude of the probability current. For reflected flow, $\overline{J}_j^{(h)}$ and $\overline{P}_j$ can be defined similarly. When region $j$ corresponds to real $p_{j,x}$, we have $J_j^{(h)} = 2k_j |t_j^{(h)}|^2 |h(\chi_j^{(h)})^\dagger \boldsymbol{\sigma} \chi_j^{(h)}|$, where

$$(\chi_j^{(h)})^\dagger \boldsymbol{\sigma} \chi_j^{(h)} = h(\sin\theta_j \cos\varphi_j, \sin\theta_j \sin\varphi_j, \cos\theta_j),$$

i.e., $|h(\chi_j^{(h)})^\dagger \boldsymbol{\sigma} \chi_j^{(h)}| = 1$. Thus

$$\begin{aligned} P_j &= (|t_j^{(+)}|^2 - |t_j^{(-)}|^2)/(|t_j^{(+)}|^2 + |t_j^{(-)}|^2), \\ \overline{P}_j &= (|r_j^{(+)}|^2 - |r_j^{(-)}|^2)/(|r_j^{(+)}|^2 + |r_j^{(-)}|^2). \end{aligned} \tag{S1.14}$$

When region $j$ corresponds to imaginary $p_{j,x}$, it no longer has a well-defined helicity (the operator $\hat{h}$ is non-Hermitian and non-unitary). In this case, the helicity polarization is not calculated.

For the electrostatic potential case, since incidence in an evanescent wave mode will not be taken into account, i.e., $p_{1,x}$, $p_y$, and $p_z$ are real, the incident state are restrained accordingly. Based on the propagation mode of Dirac fermions, $V_j < V_-$ and $V_j > V_+$ with $V_\pm = E \pm \sqrt{p_y^2 + p_z^2 + m^2}$ correspond to real $p_{j,x}$ propagating along $x$-axis in a traveling wave mode with positive and negative energy, respectively [2, 3]. And $V_- < V_j < V_+$ corresponds to imaginary $p_{j,x}$ propagating in an evanescent wave mode. Distinctly, the Klein tunneling process belongs to $V_j > V_+$. Once the region $n$ follows $V_- < V_n < V_+$, we have $T^{(+)} = T^{(-)} = 0$ and $R^{(+)} + R^{(-)} = 1$.

For the mass potential case, $U_- < U_j < U_+$ with $U_\pm = -m \pm \sqrt{E^2 - p_y^2 - p_z^2}$ corresponds to real $p_{j,x}$ propagating in a traveling wave mode, and $U_j \notin (U_-, U_+)$ corresponds to imaginary $p_{j,x}$ propagating in an evanescent wave mode. Now the parameters are $p_j = \sqrt{E^2 - (m + U_j)^2}$, $k_j = p_j/(E + m + U_j)$, and $\varphi_j = \cos^{-1}\left(\sqrt{p_j^2 - p_y^2 - p_z^2} \Big/ p_j \sin\theta_j\right)$.

### B. Numerical result vs analytical result for a linear electrostatic potential

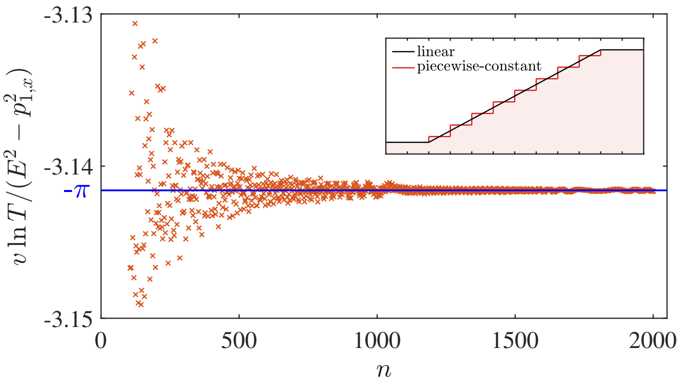


FIG. S1. The ratio of $v \ln T$ and $E^2 - p_{1,x}^2$ for piecewise-constant electrostatic potentials with $n$ regions, at $E = 2m$, $V_n = 10m$, $V_n/L = 0.01m^2$, and random incident angle parameters $(\theta_1, \varphi_1)$. Note that the difference between the ratio and $-\pi$ already falls into the range of 0.01 for $n \sim 100$. Inset shows the linear electrostatic potential and the approximation by a piecewise-constant potentials with, for example, $n = 10$.

In 1931, Sauter calculated the transmission probability for (3+1)-dimensional massive Dirac fermions under a smooth linear electrostatic potential of the form

$$V(x) = vx, 0 < x < L, \tag{S1.15}$$

with $V(x) = 0$ for $x < 0$, $V(x) = vL$ for $x > L$, and the linear slope $v$. With the appropriate hypergeometric functions, Sauter obtained an analytical expression for the transmission and reflection probabilities $T$ and $R$. For weak electric fields, there is a simple result

$$R \simeq 1, \; T = \exp\left[-\pi c(m^2c^2 + p_y^2 + p_z^2)/\hbar v\right], \tag{S1.16}$$

in the limit of $v \ll (m^2c^2 + p_y^2 + p_z^2)c/\hbar$ [4].

As a test, we compare the numerical result to Eq. (S1.16) to ensure that our numerical method is correct, and the numerical results for one-dimensional piecewise-constant electrostatic potential with enough stages fits the real solution for the smooth potential within the margin of error.

As a test of our numerical procedure, we divide the linear potential into $(n-2)$ equal portions, and then numerically solve this piecewise-constant electrostatic potential with $n$ stages and compare the transmission probability $T$. In other words, the transmission probability $T = T^{(+)} + T^{(-)}$ should approach $\exp\left[-\pi(E^2 - p_{1,x}^2)/v\right]$ in the condition of $v = V_n/L \ll E^2 - p_{1,x}^2$. Or the ratio of $v \ln T$ and $E^2 - p_{1,x}^2$ will gradually approach the constant $-\pi$ as $n$ increases, which is equivalent to Eq. (S1.16). This is indeed the case, as shown in Fig. S1, that as $n$ becomes larger and larger, the data points for different $n$ approach to $-\pi$ consistently.

## II. ANALYTICAL SOLUTION OF THE MODEL WITH 3 REGIONS

To gain insights, we solve the three region case ($n = 3$) analytically by the above method. The expressions for the overall reflection and transmission coefficients are

$$\begin{aligned}
r_1^{(+)} &= \mathrm{i}e^{-\mathrm{i}\varphi_1}(A_3C_2 - A_4C_1)/(A_2A_3 - A_1A_4),\\
r_1^{(-)} &= \mathrm{i}e^{-\mathrm{i}\varphi_1}(A_3C_4 - A_4C_3)/(A_2A_3 - A_1A_4),\\
t_3^{(+)} &= -OA_4/(A_2A_3 - A_1A_4),\\
t_3^{(-)} &= OA_3/(A_2A_3 - A_1A_4),
\end{aligned} \tag{S2.17}$$

where

$$O = 4e^{\mathrm{i}(\varphi_1/2+\varphi_3/2-\lambda_3 L\rho_3)}k_1k_2\cos\varphi_1\cos\varphi_2, \tag{S2.18}$$

and the other ones are

$$\begin{aligned}
A_1 &= e^{\mathrm{i}\varphi_3}(h_2 + e^{\mathrm{i}\varphi_1}g_{+,-}\sin\frac{\theta_3}{2}/\sin\frac{\theta_1}{2}) + e^{\mathrm{i}\varphi_1}h_1 + g_{+,+}\cos\frac{\theta_3}{2}/\cos\frac{\theta_1}{2},\\
A_2 &= e^{\mathrm{i}\varphi_3}(h_3 + e^{\mathrm{i}\varphi_1}g_{-,-}\cos\frac{\theta_3}{2}/\sin\frac{\theta_1}{2}) - e^{\mathrm{i}\varphi_1}h_4 - g_{-,+}\sin\frac{\theta_3}{2}/\cos\frac{\theta_1}{2},\\
A_3 &= e^{\mathrm{i}\varphi_3}(h_4 + e^{\mathrm{i}\varphi_1}g_{-,-}\sin\frac{\theta_3}{2}/\cos\frac{\theta_1}{2}) - e^{\mathrm{i}\varphi_1}h_3 - g_{-,+}\cos\frac{\theta_3}{2}/\sin\frac{\theta_1}{2},\\
A_4 &= e^{\mathrm{i}\varphi_3}(h_1 + e^{\mathrm{i}\varphi_1}g_{+,-}\cos\frac{\theta_3}{2}/\cos\frac{\theta_1}{2}) + e^{\mathrm{i}\varphi_1}h_2 + g_{+,+}\sin\frac{\theta_3}{2}/\sin\frac{\theta_1}{2},\\
C_1 &= e^{\mathrm{i}\varphi_3}(e^{\mathrm{i}\varphi_1}h_2 - g_{+,-}\sin\frac{\theta_3}{2}/\sin\frac{\theta_1}{2}) - h_1 + e^{\mathrm{i}\varphi_1}g_{+,+}\cos\frac{\theta_3}{2}/\cos\frac{\theta_1}{2},\\
C_2 &= e^{\mathrm{i}\varphi_3}(e^{\mathrm{i}\varphi_1}h_3 - g_{-,-}\cos\frac{\theta_3}{2}/\sin\frac{\theta_1}{2}) + h_4 - e^{\mathrm{i}\varphi_1}g_{-,+}\sin\frac{\theta_3}{2}/\cos\frac{\theta_1}{2},\\
C_3 &= e^{\mathrm{i}\varphi_3}(e^{\mathrm{i}\varphi_1}h_4 - g_{-,-}\sin\frac{\theta_3}{2}/\cos\frac{\theta_1}{2}) + h_3 - e^{\mathrm{i}\varphi_1}g_{-,+}\cos\frac{\theta_3}{2}/\sin\frac{\theta_1}{2},\\
C_4 &= e^{\mathrm{i}\varphi_3}(e^{\mathrm{i}\varphi_1}h_1 - g_{+,-}\cos\frac{\theta_3}{2}/\cos\frac{\theta_1}{2}) - h_2 + e^{\mathrm{i}\varphi_1}g_{+,+}\sin\frac{\theta_3}{2}/\sin\frac{\theta_1}{2},
\end{aligned} \tag{S2.19}$$

with

$$\begin{aligned}
h_1 &= -\mathrm{i}\cos\frac{\theta_3}{2}\sin(p_{2,x}L)[k_2^2 + k_1k_3 - k_2(k_1+k_3)\cos\theta_2]/\sin\theta_2\sin\frac{\theta_1}{2},\\
h_2 &= -\mathrm{i}\sin\frac{\theta_3}{2}\sin(p_{2,x}L)[k_2^2 + k_1k_3 + k_2(k_1+k_3)\cos\theta_2]/\sin\theta_2\cos\frac{\theta_1}{2},\\
h_3 &= -\mathrm{i}\cos\frac{\theta_3}{2}\sin(p_{2,x}L)[k_2^2 - k_1k_3 + k_2(k_1-k_3)\cos\theta_2]/\sin\theta_2\cos\frac{\theta_1}{2},\\
h_4 &= -\mathrm{i}\sin\frac{\theta_3}{2}\sin(p_{2,x}L)[k_2^2 - k_1k_3 - k_2(k_1-k_3)\cos\theta_2]/\sin\theta_2\sin\frac{\theta_1}{2},
\end{aligned} \tag{S2.20}$$

and

$$\begin{aligned}
g_{+,\pm} &= k_2(k_1+k_3)\cos(p_{2,x}L \pm \varphi_2),\\
g_{-,\pm} &= k_2(k_1-k_3)\cos(p_{2,x}L \pm \varphi_2).
\end{aligned} \tag{S2.21}$$

For coefficients $t_2^{(h)}$ and $r_2^{(h)}$, the expression can be obtained by

$$\begin{pmatrix} t_2^{(+)} \\ t_2^{(-)} \\ r_2^{(+)} \\ r_2^{(-)} \end{pmatrix} = D_2^{-1}\cdot M_2^{-1}\cdot T\cdot\begin{pmatrix} t_3^{(+)} \\ t_3^{(-)} \end{pmatrix} \tag{S2.22}$$

with $M_2^{-1}$ given by Eq. (S1.12).

For transmitted flow in region $j$ $(=2,3)$, the transformation of the helicity combination can be expressed as a matrix $\mathcal{M}$, which is determined by $\psi_1$ and the potential parameters. By the transfer matrix method, the continuity conditions in the case of an arbitrary $P_1$ can be simplified as

$$\begin{pmatrix} t_j^{(+)} \\ t_j^{(-)} \\ r_j^{(+)} \\ r_j^{(-)} \end{pmatrix} = \mathcal{T}_{1\to j} \begin{pmatrix} t_1^{(+)} \\ t_1^{(-)} \\ r_1^{(+)} \\ r_1^{(-)} \end{pmatrix} \tag{S2.23}$$

with $\mathcal{T}_{1\to j} = D_j^{-1} \cdot M_j^{-1} \cdot H_{j-1}^{-1} \cdots H_3^{-1} \cdot H_2^{-1} \cdot I$ a $4\times 4$ matrix, and $r_j^{(+)} = r_j^{(-)} = 0$ for $j=3$.

The first two rows and the first two columns of $\mathcal{T}_{1\to j}$ form the non-unitary matrix $\mathcal{M}$. If we only concern the redistribution rule of helicity, we may neglect the common phase of the transmission or reflection coefficients and add a normalization constant, which does not affect the helicity. To be specific, we can define a unitary matrix $|\mathcal{M}|^{-1/2}\mathcal{M}$, where $|\mathcal{M}|^{-1/2}$ is the normalization coefficient. More importantly, $|\mathcal{M}|^{-1/2}\mathcal{M}$ as a transformation between two sets of the normalized transmitted coefficients is process-independent, simplified as

$$\begin{pmatrix} t_j^{(+)} \\ t_j^{(-)} \end{pmatrix} = |\mathcal{M}|^{-1/2} \begin{pmatrix} \mathcal{M}_{(+,+)} & \mathcal{M}_{(+,-)} \\ \mathcal{M}_{(-,+)} & \mathcal{M}_{(-,-)} \end{pmatrix} \cdot \begin{pmatrix} t_1^{(+)} \\ t_1^{(-)} \end{pmatrix} \tag{S2.24}$$

where

$$\mathcal{M}_{(h',h)} = \langle \psi_j^{(h')} | \, \alpha_x \, | \psi_1^{(h)} \rangle \,, \tag{S2.25}$$

with normalized ket $|\psi_j^{(h)}\rangle = \psi_j^{(h)}/|\psi_j^{(h)}|$, and

$$|\mathcal{M}|^{-1/2} = \sqrt{(k_1^2+1)(k_j^2+1)/\left(k_1^2+k_j^2+2k_1k_j[\cos(\varphi_1+\varphi_j)\sin\theta_1\sin\theta_j - \cos\theta_1\cos\theta_j]\right)}.$$

Notably, when the incident wavefunction $\psi_1$ is given, from Eq. (S1.2), $|\psi_j^{(h')}\rangle$ is solely determined by the potential height $V_j$ in region $j$, then from Eq. (S2.25), the unitary transformation matrix $|\mathcal{M}|^{-1/2}\mathcal{M}$ is also determined. The introduction of $|\mathcal{M}|^{-1/2}$ can simultaneously eliminate the effects of the process-dependent phase and probability current. In other words, there is a universal helicity redistribution rule in the actual tunneling process, which is process-independent. Since $\begin{pmatrix} t_j^{(+)} \\ t_j^{(-)} \end{pmatrix}$ is a normalized vector, Eq. (S2.24) actually characters the transformation from $|\psi_1\rangle$ to $|\psi_j\rangle$, where $|\psi_j\rangle = \psi_j/|\psi_j|$ is the final spinor state vector in the transport process, with an process-dependent unobservable common phase factor disregarded.

## III. THE UNIVERSAL HELICITY REDISTRIBUTION RULE IN THE ELECTROSTATIC POTENTIAL CASE

Since the unitary transformation matrix $|\mathcal{M}|^{-1/2}\mathcal{M}$ is process-independent, there is a universal helicity redistribution rule in transport under the piecewise-constant electrostatic potential.

### A. The rule dictated by one-parameter transformation group of Lorentz boost $\Lambda(w)$

The energy $E$, $y$-momentum $p_y$, and $z$-momentum $p_z$ are conserved in the whole tunneling process. For a given initial state $|\psi_1\rangle$, the transport process resulting the final normalized state $|\psi_j\rangle$ of the transmitted part in region $j$ can be regarded as an

abstract operation $g$ on the Hilbert space of Dirac spinors, that maps $|\psi_1\rangle$ to $|\psi_j\rangle$. It turns out that $g$ only depends on the electrostatic potential $V_j$ in this region, when the initial state $|\psi_1\rangle$ (parameterized by $E$, $p_y$, $p_z$, $t_1^{(+)}$, $t_1^{(-)}$) is given, as can be demonstrated with the help of $|\mathcal{M}|^{-1/2}\mathcal{M}$. All possible operations form a set $\mathcal{G} = \{g\}$. The multiplication of two operations $g_2 \circ g_1$ can be defined as the combined process: the Dirac fermions transport first from region 1 with $V_1 = 0$ and $|\psi_1\rangle$ to region $j$ with $V_j$ and $|\psi_j\rangle$, and then from region $j$ with now the initial state being $|\psi_j\rangle$ to region $k$ with $V_k$ and $|\psi_k\rangle$. It is straightforward to show that $\left[|\mathcal{M}|^{-1/2}\mathcal{M}\right]_{k\leftarrow j}\left[|\mathcal{M}|^{-1/2}\mathcal{M}\right]_{j\leftarrow 1} = \left[|\mathcal{M}|^{-1/2}\mathcal{M}\right]_{k\leftarrow 1}$.

For simplicity, for a given initial state, we denote the transformation $|\mathcal{M}|^{-1/2}\mathcal{M}$ in Eq. (S2.24) as $\mathcal{M}_{j1}$ with a single parameter $\Delta V \equiv V_j - V_1 = V_j$.

- (closure) If there is an element $g_1$ corresponding to $\mathcal{M}_{j1}(\Delta V = V_j)$, and another $g_2$ corresponding to $\mathcal{M}_{kj}(\Delta V = V_k - V_j)$. Then there exists $g_3 \in \mathcal{G}$ associated with $\mathcal{M}_{k1}(\Delta V = V_k) = \mathcal{M}_{kj} \cdot \mathcal{M}_{j1}$, i.e., $g_2(V_k - V_j) \circ g_1(V_j) = g_3(V_k)$. Thus the operations are additive with respect to the electrostatic potential $V$ and consequently $g_2 \circ g_1 = g_1 \circ g_2$.
- (associative law) The matrix multiplication satisfies the associative law.
- (identity element) The identity element $e$ corresponds to $\mathcal{M}_{j1}(\Delta = 0) = \mathbb{1}_2$.
- (inverse element) Assume an arbitrary element $g$ corresponding to $\mathcal{M}_{j1}(\Delta V = V_j)$. There exists $g^{-1} \in \mathcal{G}$ corresponding to $\mathcal{M}_{1j}(\Delta V = -V_j)$.

Therefore, $(\mathcal{G}, \circ)$ forms a one-parameter transformation group. The set of $\{\mathcal{M}_{j1}\}$ forms a two-dimensional representation of this group, where $\mathcal{M}_{j1}$ depends on $(E, p_y, p_z)$ and $V_j$. According to the effective energy-momentum relation, we find out a more general one-parameter representation for this group, i.e., the Lorentz boost $\Lambda(w)$ along the $x$-axis with rapidity $w$ for $V_j < V_-$, and for $V_j > V_+$ this group is a combined Lorentz boost $\Lambda(\mathrm{i}\pi)\Lambda(w)$ along the $x$-axis. This kind of complex Lorentz boost has been used before to represent negative energy modes in massive Thirring model [5, 6], prove the $\mathcal{PCT}$ theorem by Jost in 1957 [7], and expose the intimate connection between $\mathcal{PCT}$ and Lorentz symmetry [7–9].

For $V_j < V_-$, the one-parameter $w$ is determined by the following energy-momentum transformation

$$\begin{pmatrix} E - V_j \\ p_{j,x} \end{pmatrix} = \begin{pmatrix} \cosh w & -\sinh w \\ -\sinh w & \cosh w \end{pmatrix} \cdot \begin{pmatrix} E \\ p_{1,x} \end{pmatrix}, \tag{S3.26}$$

where the rapidity $w$ is defined by $\cosh w = (1 - v^2)^{-1/2}$ with $v$ being the relative velocity of the two inertial frames $O$ with $p_{1,x}$ and $O'$ with $p_{j,x}$. Using four-vector $x^\mu = (x^0, x^1, x^2, x^3) = (t, \mathbf{x})$ for the description of the space-time coordinates, we select the Minkowski metric $g_{\mu\nu} = \mathrm{diag}(1, -1, -1, -1)$. In $O$, the free Dirac equation in covariance formulation is

$$(\mathrm{i}\gamma^\mu \partial_\mu - m)\psi(x) = 0, \tag{S3.27}$$

with definitions $\gamma^0 = \beta$, $\gamma^i = \beta\alpha_i$, and the partial derivative $\partial_\mu \equiv \partial/\partial x^\mu$.

The linear transformation between $\psi(x)$ and $\psi'(x')$ can be constructed as

$$\psi'(x') = \hat{S}[\Lambda(w)]\psi(\Lambda^{-1}x') = \hat{S}[\Lambda(w)]\psi(x) \tag{S3.28}$$

under a finite proper Lorentz transformation $\Lambda(w)$, where the operator $\hat{S}[\Lambda(w)]$ is the spinor representation of the Lorentz boost $\Lambda(w)$. Note that in general $\hat{S}[\Lambda(w)]$ is not unitary [10]. Since form invariance of the Dirac equations of motion is required, $\hat{S}$ must have the property

$$\gamma^\nu = \hat{S}\gamma^\mu \hat{S}^{-1}\Lambda^\nu{}_\mu. \tag{S3.29}$$

Thus the operator $\hat{S}$ for $\Lambda(w)$ can be obtained by solving corresponding infinitesimal Lorentz transformations $\Lambda_{\text{inf}}$, written as

$$\hat{S}_{\text{inf}} = \exp[(\mathrm{i}/4)w\hat{\sigma}_{\mu\nu}(\hat{I}_n)^{\mu\nu}] \tag{S3.30}$$

with the matrix $\hat{\sigma}_{\mu\nu} = (\mathrm{i}/2)[\gamma_\mu, \gamma_\nu]_-$ and generator $(\hat{I}_n)^\mu{}_\nu$ corresponding to $\Lambda_{\text{inf}}$ for Lorentz group, including $\hat{I}_x, \hat{I}_y, \hat{I}_y$ for the Lorentz transformation into a moving system and $\hat{I}_1, \hat{I}_2, \hat{I}_3$ for spatial rotations. Since this Lorentz boost $\Lambda(w)$ is along the $x$-axis, we have

$$\hat{S}[\Lambda(w)] = e^{-\alpha_x w/2} = \cosh(w/2)\mathbb{1}_4 - \sinh(w/2)\alpha_x, \tag{S3.31}$$

where $\mathbb{1}_4$ is the $4 \times 4$ identity matrix.

It is straightforward to show that, the normalized spinor state $|\psi'\rangle = \zeta\hat{S}\,|\psi_1\rangle$ obtained by $\hat{S}$ in $O'$ is the same as the final state $|\psi_j\rangle$ in the actual transport process, where $\zeta = [\cosh w - 2k_1 \sinh w \sin\theta_1 \cos\varphi_1/(1+k_1^2)]^{-1/2}$ is the normalization coefficient. Besides, the final state $|\psi_j\rangle$ is a linear combination of $|\psi_j^{(h)}\rangle$, i.e., $|\psi_j\rangle = \zeta\hat{S}\,|\psi_1\rangle = \sum_h t_j^{(h)}\,|\psi_j^{(h)}\rangle$, where $t_j^{(h)}$ has been normalized. The linear combination coefficient follows $t_j^{(h)} = \langle\psi_j^{(h)}|\psi_j\rangle = \zeta\,\langle\psi_j^{(h)}|\,\hat{S}\,|\psi_1\rangle$, expressed as

$$\begin{pmatrix} t_j^{(+)} \\ t_j^{(-)} \end{pmatrix} = \mathcal{L}(w)\cdot\begin{pmatrix} t_1^{(+)} \\ t_1^{(-)} \end{pmatrix} = \zeta\begin{pmatrix} \langle\psi_j^{(+)}| \\ \langle\psi_j^{(-)}| \end{pmatrix}\hat{S}[\Lambda(w)]\begin{pmatrix} |\psi_1^{(+)}\rangle & |\psi_1^{(-)}\rangle \end{pmatrix}\cdot\begin{pmatrix} t_1^{(+)} \\ t_1^{(-)} \end{pmatrix}. \tag{S3.32}$$

Utilizing Eq. (S3.26), we have

$$\tanh\frac{w}{2} = \frac{\sinh w}{\cosh w + 1} = \frac{k_1 e^{\mathrm{i}\varrho_1} - k_j e^{\mathrm{i}\varrho_j}}{1 - k_1 k_j e^{\mathrm{i}(\varrho_1+\varrho_j)}} \tag{S3.33}$$

with $\varrho_j = \cos^{-1}(\sin\theta_j\cos\varphi_j)$, then it is easy to prove that the $2\times 2$ matrix $\mathcal{L}(w)$ equals $|\mathcal{M}|^{1/2}\mathcal{M}$, i.e., Eq. (S3.32) is the same as Eq. (S2.24).

Therefore, the one-parameter transformation group dictating the spinor transformation of Dirac fermions in transport through electrostatic potentials is just the Lorentz boost with a more abstracted parameter, i.e., rapidity $w$, instead of the detailed parameters $(E, p_y, p_z)$ and $V_j$ in the direct two-dimensional representation $|\mathcal{M}|^{1/2}\mathcal{M}$.

The ratio of the two helicity components for the final state $|\psi_j\rangle$ is then

$$t_j^{(+)}/t_j^{(-)} = \frac{k_1+k_j}{k_1-k_j}\cdot\frac{\tan(\theta_j/2)e^{-\mathrm{i}\varphi_j} + \tan(\theta_1/2)e^{\mathrm{i}\varphi_1}}{e^{-\mathrm{i}\varphi_j} - \tan(\theta_1/2)\tan(\theta_j/2)e^{\mathrm{i}\varphi_1}}. \tag{S3.34}$$

Based on Eq. (S1.14), we have

$$P_j = (\eta_j - 1)/(\eta_j + 1), \tag{S3.35}$$

where

$$\eta_j = \left|t_j^{(+)}/t_j^{(-)}\right|^2 = \left(\frac{k_1+k_j}{k_1-k_j}\right)^2\cdot\frac{1+\cos(\varrho_1+\varrho_j)}{1-\cos(\varrho_1+\varrho_j)}. \tag{S3.36}$$

Based on Eqs. (S3.35) and (S3.36), for $P_1 = 1$, the helicity polarization $P_j$ is determined only by the physical quantities $(E, \mathbf{p}_1)$ and $V_j$. Alternatively, due to the rotational symmetry with respect to the $x$-axis, $P_j$ is solely determined by ($E$, $\varrho_1$, $V_j$). For reflected flow, one only needs to change $\varrho_j$ to $\pi - \varrho_j$ to obtain the corresponding helicity polarization $\overline{P}_j$.

### B. The rule in Klein tunneling regime dictated by complex Lorentz boost $\Lambda(\mathrm{i}\pi)\Lambda(w)$

For $V_j > V_+$ (Klein tunneling regime), we have $E - V_j < 0$ and $\pi/2 < \varphi_j < \pi$. Conventional Lorentz boost $\Lambda(w)$ with real $w$ fails to link the positive and negative energy states, i.e, Eq. (S3.26) has no real solution when $E - V_j < 0$. Interestingly, by

replacing $w$ with $\mathrm{i}\pi$, the operation $\Lambda(\mathrm{i}\pi)$ flips the sign of the effective energy and $p_x$. The complex Lorentz boost $\Lambda(\mathrm{i}\pi)$ can be a great bridge to realize the one-to-one mapping from $V_j < V_-$ regime to $V_j > V_+$ regime, donated as the transformation from $O'$ to $\widetilde{O}$ in Fig. 2 of the main text. Thus we consider the combined operation $\Lambda(\mathrm{i}\pi)\Lambda(w)$: $O \xrightarrow{\Lambda(w)} O' \xrightarrow{\Lambda(\mathrm{i}\pi)} \widetilde{O}$, whose spinor representation is

$$\hat{S}[\Lambda(\mathrm{i}\pi)]\hat{S}[\Lambda(w)] = -\mathrm{i}\cosh(w/2)\alpha_x + \mathrm{i}\sinh(w/2)\mathbb{1}_4. \tag{S3.37}$$

Indeed, $\hat{S}[\Lambda(\mathrm{i}\pi)]$ will flip the helicity of the spinor state vector. Taking the case of the state vector $|\psi^{(+)}(E,\theta,\varphi)\rangle$ with positive helicity, energy $E$, and angle parameters $(\theta,\varphi)$ of the momentum, we have

$$\begin{aligned}\hat{S}[\Lambda(\mathrm{i}\pi)]\,|\psi^{(+)}(E,\theta,\varphi)\rangle &= -\mathrm{i}\alpha_x\frac{1}{\sqrt{1+k^2}}\begin{pmatrix}\cos\frac{\theta}{2}e^{-\mathrm{i}\varphi/2}\\ \sin\frac{\theta}{2}e^{\mathrm{i}\varphi/2}\\ k\cos\frac{\theta}{2}e^{-\mathrm{i}\varphi/2}\\ k\sin\frac{\theta}{2}e^{\mathrm{i}\varphi/2}\end{pmatrix} = \frac{1}{\sqrt{1+k'^2}}\begin{pmatrix}-\sin\frac{\theta}{2}e^{-\mathrm{i}(\pi-\varphi)/2}\\ \cos\frac{\theta}{2}e^{\mathrm{i}(\pi-\varphi)/2}\\ k'\sin\frac{\theta}{2}e^{-\mathrm{i}(\pi-\varphi)/2}\\ -k'\cos\frac{\theta}{2}e^{\mathrm{i}(\pi-\varphi)/2}\end{pmatrix}\\ &= |\psi^{(-)}(-E,\theta,\pi-\varphi)\rangle\,,\end{aligned}$$

where $k = p/(E+m)$ and $k' = p/(-E+m)$. Similar to the case of $V_j < V_-$, the normalized spinor state $|\widetilde{\psi}\rangle = \zeta\hat{S}[\Lambda(\mathrm{i}\pi)]\hat{S}[\Lambda(w)]\,|\psi_1\rangle$ in $\widetilde{O}$ is the same as the final state $|\psi_j\rangle$ in the actual Klein tunneling process. Besides,

$$\begin{aligned}\mathcal{L}(w) &= \zeta\begin{pmatrix}\langle\psi_j^{(+)}|\\ \langle\psi_j^{(-)}|\end{pmatrix}\hat{S}[\Lambda(\mathrm{i}\pi)]\hat{S}[\Lambda(w)]\begin{pmatrix}|\psi_1^{(+)}\rangle & |\psi_1^{(-)}\rangle\end{pmatrix}\\ &= |\mathcal{M}|^{1/2}\mathcal{M},\end{aligned} \tag{S3.38}$$

which is the same as Eq. (S2.24). Therefore, the combined Lorentz boost $\Lambda(\mathrm{i}\pi)\Lambda(w)$ perfectly describes the operation from $|\psi_1\rangle$ to $|\psi_j\rangle$ in the actual Klein tunneling process.

For reflected flow in region $j\ (=1,2)$ following $\overline{\psi}_j = r_j^{(h)}\overline{\psi}_j^{(h)}$, we have a similar form as Eq. (S2.24-S3.32) except that now $\mathcal{M}_{(h',h)} = -\langle\overline{\psi}_2^{(h')}|\,\alpha_x\,|\psi_1^{(h)}\rangle$ for $j=2$ and $\mathcal{M}_{(h',h)} = \langle\overline{\psi}_1^{(h')}|\psi_1^{(h)}\rangle$ for $j=1$ in Eq. (S2.24), $p_{j,x}$ replaced by $-p_{j,x}$ in Eq. (S3.26), and $\langle\psi_j^{(h)}|$ replaced by $\langle\overline{\psi}_j^{(h)}|$ in Eq. (S3.32).

In the end, we introduce the spinor representation $\mathcal{P}_x$ of the mirror reflection operator $a$ in the $y-z$ plane, denoted as $\hat{S}(a) = \mathcal{P}_x$. The operator $a$ is

$$a^\mu{}_\nu = \begin{pmatrix}1 & 0 & 0 & 0\\ 0 & -1 & 0 & 0\\ 0 & 0 & 1 & 0\\ 0 & 0 & 0 & 1\end{pmatrix},$$

and $\mathcal{P}_x$ holds also the defining equation (S3.29)

$$\begin{aligned}a^\mu{}_\nu\gamma^\nu &= \mathcal{P}_x\gamma^\mu\mathcal{P}_x^{-1}\\ a^\sigma{}_\mu a^\mu{}_\nu\gamma^\nu &= \delta^\sigma_\nu\gamma^\nu = \mathcal{P}_x a^\sigma{}_\mu\gamma^\mu\mathcal{P}_x^{-1}\end{aligned} \tag{S3.39}$$

with the simple solution $\mathcal{P}_x = e^{\mathrm{i}\phi_x}\gamma^0\gamma^2\gamma^3$, where for the time being $\phi_x$ is an unobservable arbitrary phase. For parity operator $\mathcal{P}$, $\mathcal{P} = e^{\mathrm{i}\phi_\mathcal{P}}\gamma^0 = \mathcal{P}_y\mathcal{P}_z\mathcal{P}_x$ with $e^{\mathrm{i}\phi_\mathcal{P}} = \pm1, \pm\mathrm{i}$ since that four space inversions will reproduce the spinor. Denoting the subscript of mirror reflection operator as $x, y, z = 1, 2, 3$, we have $\mathcal{P}_i = e^{\mathrm{i}\phi_i}\gamma^0\varepsilon_{ijk}\gamma^j\gamma^k$ with $i \neq j \neq k$ and Levi-Civita symbol $\varepsilon_{ijk}$. Thus $e^{\mathrm{i}(\phi_1+\phi_2+\phi_3)} = e^{\mathrm{i}\phi_\mathcal{P}}$, and $\phi_i$ belongs to the same value range for arbitrary $i$, i.e., $e^{\mathrm{i}\phi_i} = \pm1, \pm\mathrm{i}$.

Besides, $\mathcal{C}$ and $\mathcal{T}$ are the spinor representations of the charge conjugate operator and the time-reversal operator, respectively, following

$$\begin{aligned}\mathcal{C} &= \mathrm{i}\gamma^2\mathcal{K},\\ \mathcal{T} &= \mathrm{i}\gamma^1\gamma^3\mathcal{K},\end{aligned} \tag{S3.40}$$

where $\mathcal{K}$ denotes complex conjugation. Thus

$$\begin{aligned}\mathcal{P}_x\mathcal{C}\mathcal{T} &= e^{\mathrm{i}\phi}\gamma^0\gamma^2\gamma^3\mathrm{i}\gamma^2\mathcal{K}(\mathrm{i}\gamma^1\gamma^3\mathcal{K})\\ &= e^{\mathrm{i}\phi}\gamma^0\gamma^2\gamma^3\mathrm{i}\gamma^2(\mathrm{i}\gamma^1\gamma^3\mathcal{K})^*\\ &= e^{\mathrm{i}\phi}\gamma^0\gamma^2\gamma^3\gamma^2\gamma^1\gamma^3\\ &= e^{\mathrm{i}\phi}\alpha_x,\end{aligned} \tag{S3.41}$$

which equals to $\hat{S}[\Lambda(\mathrm{i}\pi)] = -\mathrm{i}\alpha_x$ disregarding an unobservable phase.

## IV. THE UNIVERSAL HELICITY REDISTRIBUTION RULE IN THE MASS POTENTIAL CASE DICTATED BY $\Gamma(\mu)$

Similarly, for the mass potential case, we can obtain that the transformation $|\mathcal{M}|^{-1/2}\mathcal{M}$ between two sets of the normalized transmitted coefficients is also process-independent, which has the form Eq. (S2.24) where $\psi_j^{(h)}$, $k_j$, $\theta_j$, and $\varphi_j$ change accordingly. And we denote the transformation $|\mathcal{M}|^{-1/2}\mathcal{M}$ as $\mathcal{M}_{j1}$ with a single parameter $\Delta U \equiv U_j - U_1 = U_j$. By regarding the transformation from $|\psi_1\rangle$ with given $(E, m, p_y, p_z)$ to $|\psi_j\rangle$ as an operation $g$, for $U_j \in (U_-, U_+)$, all different operations form a set $\mathcal{G} = \{g\}$. And $(\mathcal{G}, \circ)$ with "$\circ$" having the same meaning as in the electrostatic potential case, is a one-parameter transformation group denoted as $\Gamma(\Delta U)$, which has a two-dimensional representation $\{\mathcal{M}_{j1}\}$.

According to the momentum-effective mass relation, there is a parameter $\mu$ independent of the initial state to character this group, denoted as $\Gamma(\mu)$. The one-parameter $\mu$ represents the rotation angle in the plane of effective mass $m + U_j$ and $x$-momentum, following

$$\begin{pmatrix} m + U_j \\ p_{j,x} \end{pmatrix} = \begin{pmatrix} \cos\mu & -\sin\mu \\ \sin\mu & \cos\mu \end{pmatrix} \cdot \begin{pmatrix} m \\ p_{1,x} \end{pmatrix}, \tag{S4.42}$$

and the spinor representation of the group $\Gamma(\mu)$ is a $4 \times 4$ unitary matrix

$$\hat{S}_m[\Gamma(\mu)] = \cos(\mu/2)\mathbb{1}_4 - \sin(\mu/2)\beta\alpha_x. \tag{S4.43}$$

In this regard, the Lorentz boost $\Lambda(w)$ represents a pseudo-rotation in the $(E, p_x)$ plane with the premise of the conservation of the distance between two space-time points in Minkowski space. And the group $\Gamma(\mu)$ represents a rotation in the $(m+U, p_x)$ plane with the premise of the conservation of energy.

Notably, the parameter $\mu$ has the meaning of the rotation angle, thus $\hat{S}_m[\Gamma(4\pi)] = \mathbb{1}_4$ due to the characteristic of the spinor. And $\hat{S}_m[\Gamma(\mu)]$ with $\mu = [0, 4\pi)$ forms a matrix group, which leads to the multi-solution problem of Eq. (S4.42) when we determine the value of $\mu$ in an actual tunneling process. To solve the the multi-solution problem and ensure the consistency of the form

$$\mathcal{L}_m = \begin{pmatrix} \langle\psi_j^{(+)}| \\ \langle\psi_j^{(-)}| \end{pmatrix} \hat{S}_m[\Gamma(\mu)] \begin{pmatrix} |\psi_1^{(+)}\rangle & |\psi_1^{(-)}\rangle \end{pmatrix} = |\mathcal{M}|^{1/2}\mathcal{M},$$

we require that $\mu \in (2\pi, 4\pi)$ for $m + U_j > 0$, and $\mu \in (0, 2\pi)$ for $m + U_j < 0$.

For reflected flow in region $j$ $(= 1, 2)$, we follow the above restriction about $\mu$. In this case, $\mathcal{M}_{(h',h)} = \langle\overline{\psi}_2^{(h')}|\,\alpha_x\,|\psi_1^{(h)}\rangle$ for $j = 2$, and $\mathcal{M}_{(h',h)} = \langle\overline{\psi}_1^{(h')}|\psi_1^{(h)}\rangle - \mathrm{i}p_{1,x}|h - h'|/m(1/k_1 + k_1)$ for $j = 1$.

Generally, the helicity redistribution in the mass potential case follows a similar form of expression as in the electrostatic potential case, although the details and properties are different. However, for the reflected flow in region 1, even the form of the expression is different, as demonstrated by the expressions of $\mathcal{M}_{(h',h)}$.


[1] P. Strange, *Relativistic Quantum Mechanics: With Applications in Condensed Matter and Atomic Physics* (Cambridge University Press, Cambridge, 1998).

[2] S. De Leo and P. Rotelli, Phys. Rev. A **86**, 032113 (2012).

[3] J. Navarro-Giraldo and C. Quimbay, Ann. Phys. **412**, 168022 (2020).

[4] F. Sauter, Z. Phys. **69**, 742 (1931).

[5] H. Bergknoff and H. Thacker, Phys. Rev. D **19**, 3666 (1979).

[6] H. B. Thacker, Rev. Mod. Phys. **53**, 253 (1981).

[7] R. Jost, Helv. Phys. Acta. **30**, 153 (1957).

[8] C. D. Froggatt and H. B. Nielsen, *Origin of Symmetries* (World Scientific, Singapore, 1991) pp. 86–91.

[9] R. Lehnert, Symmetry **8**, 114 (2016).

[10] W. Greiner, *Relativistic Quantum Mechanics: Wave Equations* (Springer, Berlin, 2000).
